# Supplementary material for: A Decade of Mal-Activity Reporting: A Retrospective Analysis of Internet Malicious Activity Blacklists
Source: arXiv:1904.10629 source file (2019-04-24)
Supplement: Supplementary file 1 [file appendix.tex]

%\appendix
%\section{Unrouted IPs}
%In case when BGP routeview does not determine the corresponding ASes for IP addresses that fall in the ranges 10.0.0.0 - 10.255.255.255, 172.16.0.0 -- 172.31.255.255, 127.42.0.0 -- 127.42.255.255, or 192.168.0.0 -- 192.168.255.255, as these blocks are reserved for private internet use \cite{rfc1918}. Unfortunately, some addresses in these blocks do occur in traces since some ISPs use this address space for internal router interfaces\ik{cite}. In Table~\ref{tab:asrouting}, we show that we were unable to resolve only 0.55\% of the total unique IP addresses that correspond to malicious activities in our dataset. 
%
%\begin{table}[h!]
%\centering
%\begin{tabular}{r r l}
%\toprule
%{\bf BGP Routeview Reported Tag Name } & {\bf Count} & {\bf Description} \\
%\midrule
%ASUnrouted	& 1476 & \ik{TBD}\\
%ASprivate\_10X	& 142 & \ik{TBD}\\
%ASprivate\_100X	& 2 & \ik{TBD}\\
%\midrule
%Total Not Resolved	& 1618 & -\\
%Total Unique IPs	& 297,095 & -\\
%\midrule
%\%age of Unresolved	& 0.55\%  & -\\
%\%age of resolved	& 99.55\% & -\\
%\bottomrule
%\end{tabular}
%\caption{AS reported in BGP routeview dataset for unrouted (or unresolved) IP address. BGP routeview results in `Tag' for unrouted IP addresses.}
%\label{tab:asrouting}
%\end{table}
%
%
%\section{Attack Classes}
%In this appendix, we list reported labels that represent sub-categories of attacks or malicious activities in our dataset. We derive six different attack classes, detailed in Section~\ref{sec:mtypes}, from these sub-categories. 

%
%\section{Scatterplots}
%\begin{figure}[h!]
%\centering
%\includegraphics[width=1\columnwidth]{./new_plots/mean_life_norm_severity_scatter.png}
%\caption{Severity Analysis: Scatter relationship between Severity and Mean Lifetime. } 
%\label{Fig:results:sev_life}
%\end{figure}
%
%\begin{figure}[h!]
%\centering
%\includegraphics[width=1\columnwidth]{./new_plots/mean_death_severity_scatter.png}
%\caption{Severity Analysis: Scatter relationship between Severity and Mean Deathtime. \ben{Countries Disobey the apparent trend in ASes and IPs}} 
%\label{Fig:results:sev_death}
%\end{figure}
%
%
%\small
%
%\input{attack_labels_frequency.tex}
%\input{content_type.tex}
